# Supplementary material for: The I/O complexity of hybrid algorithms for square matrix multiplication
Source: arXiv:1904.12804 source file (2019-04-29)
Supplement: Supplementary file 1 [file appendix.tex]

\section{Proof of properties of CDAGs}
